# Supplementary material for: VideoSearch-R1: Iterative Video Retrieval and Reasoning via Soft Query Refinement
Source: arXiv:2607.00446 source file (2026-07-01)
Supplement: Supplementary file 2 [file model_size.tex]

\begin{table}[t]
\centering
\small
\setlength{\tabcolsep}{6pt}
\begin{tabular}{llcccc}
\toprule
Dataset & SQR Module & R@1 & R@5 & R@10 & R@100 \\
\midrule
\multirow{3}{*}{ActivityNet}
& Qwen3-VL-2B~\cite{bai2025qwen3} & 54.8 & 77.59 & 85.43 & 97.40 \\
& Qwen3-VL-4B~\cite{bai2025qwen3} & 54.92 & 76.59 & 84.32 & 96.99 \\
& Qwen3-VL-8B~\cite{bai2025qwen3} & \textbf{55.25} & \textbf{78.40} & \textbf{86.24} & \textbf{97.97} \\
\midrule
\multirow{3}{*}{Charades}
& Qwen3-VL-2B~\cite{bai2025qwen3} & 21.72 & 41.48 & \textbf{51.24} & 83.58 \\
& Qwen3-VL-4B~\cite{bai2025qwen3}& 21.75 & 39.06 & 48.23 & 81.75 \\
& Qwen3-VL-8B~\cite{bai2025qwen3}& \textbf{22.15} & \textbf{41.53} & 50.75 & \textbf{83.98} \\
\midrule
\multirow{3}{*}{DiDeMo}
& Qwen3-VL-2B~\cite{bai2025qwen3} & 55.49 & 78.84 & 85.17 & 96.59 \\
& Qwen3-VL-4B~\cite{bai2025qwen3} & 55.25 & 76.92 & 83.13 & 95.94 \\
& Qwen3-VL-8B~\cite{bai2025qwen3} & \textbf{55.62} & \textbf{79.22} & \textbf{85.57} & \textbf{96.96} \\
\bottomrule
\end{tabular}
\caption{Effect of rewriter model scale in the hard-query retrieval-retry setting.}
\label{tab:hqr_model_scale}
\end{table}
